# Supplementary material for: Deep Generative Models for Offline Policy Learning: Tutorial, Survey, and Perspectives on Future Directions
Source: arXiv:2402.13777 source file (2024-05-26)
Supplement: Supplementary file 1 [file 10-Appendix.tex]

\appendix
\section{Appendix}
You may include other additional sections here.
